# Supplementary material for: Closing the loop: Autonomous experiments enabled by machine-learning-based online data analysis in synchrotron beamline environments
Source: arXiv:2306.11899 source file (2023-06-20)
Supplement: Supplementary file 1 [file closed_loop_SI.pdf]

# Supporting Information - Closing the loop: Autonomous experiments enabled by machine-learning-based online data analysis in synchrotron beamline environments

LINUS PITHAN,<sup>a\*</sup> VLADIMIR STAROSTIN,<sup>a</sup> DAVID MARECEK,<sup>b</sup>  
 LUKAS PETERSDORF,<sup>c</sup> CONSTANTIN VÖLTER,<sup>a</sup> VALENTIN MUNTEANU,<sup>a</sup>  
 MACIEJ JANKOWSKI,<sup>d</sup> OLEG KONOVALOV,<sup>d</sup> ALEXANDER GERLACH,<sup>a</sup>  
 ALEXANDER HINDERHOFER,<sup>a</sup> BRIDGET MURPHY,<sup>c</sup> STEFAN KOWARIK<sup>b\*</sup> AND  
 FRANK SCHREIBER <sup>a\*</sup>

<sup>a</sup>*Universität Tübingen, Inst. für Angewandte Physik, Auf der Morgenstelle 10, 72076 Tübingen, Germany,* <sup>b</sup>*Universität Graz, Physikalische und Theoretische Chemie, Heinrichstraße 28, 8010 Graz, Austria,* <sup>c</sup>*Universität Kiel, Inst. für Experimentelle und Angewandte Physik, Leibnizstraße 19, 24118 Kiel, Germany,* and <sup>d</sup>*ESRF, The European Synchrotron, 71 avenue des Martyrs, CS 40220, 38043 Grenoble Cedex 9, France.* E-mail: *linus.pithan@uni-tuebingen.de, stefan.kowarik@uni-graz.at, frank.schreiber@uni-tuebingen.de*

machine learning; reflectometry; xrr; nr; synchrotron; autonomous experiments; closed loop control;

beamline control

At the time of the experiment BLISS 1.10 and pytango 9.3 were available on the ID10 beamline.

### SI-1. Tango device servers wrapping around ML Models

A tango device server with specific API to wrap around the ML models developed based on pytorch and tensorflow used in the context of this study.

```

1 from typing import Iterable
2 import numpy as np
3 from pprint import pprint
4
5 from tango.server import Device
6 from tango.server import run
7 from tango.server import attribute, command, device_property
8 from tango import AttrWriteType
9
10 # python code wrapping around pytorch model
11 # available on request or in follow-up publication
12 from reflectorch.inference import InferenceModel
13
14
15 def energy_to_wavelength(energy: float):
16     """Conversion from photon energy (eV) to photon wavelength (
17     angstroms)"""
18     return 1.2398 / energy * 1e4
19
20 class TorchEvaluator(Device):
21     preprocess_attributes = {
22         "beam_width": np.float64,
23         "sample_length": np.float64,
24         "energy_keV": np.float64,
25     }
26
27     input_attributes = {
28         "tth": [np.float64],
29         "intensity": [np.float64],
30         "transm": [np.float64],
31         "priors": [[np.float64]],
32         "count_time": [np.float64],
33     }
34     prediction_attributes = {
35         "q": [np.float64],
36         "q_interp": [np.float64],
37         "refl": [np.float64],
38         "refl_interp": [np.float64],
39         "refl_predicted": [np.float64],
40         "refl_predicted_polished": [np.float64],
41         "parameters": [np.float64],
42         "parameters_polished": [np.float64],
43         "parameter_names": [str],

```

```

44     "sld_profile": [np.float64],
45     "sld_x_axis": [np.float64],
46     "sld_profile_polished": [np.float64],
47 }
48
49 def __init__(self, *args, **kwargs):
50     Device.__init__(self, *args, **kwargs)
51
52     self._prefix_dict = dict()
53
54     self._input_data = self._initialize_dynamic_attributes(
55         "input", self.input_attributes
56     )
57     self._prediction_output = self._initialize_dynamic_attributes(
58         "prediction", self.prediction_attributes
59     )
60     self._preprocess_data = self._initialize_dynamic_attributes(
61         "preprocess", self.preprocess_attributes
62     )
63     self.inference_model = InferenceModel("l2q256_exp_3")
64
65 @property
66 def prediction_output(self):
67     return self._prediction_output
68
69 @command(dtype_out=int)
70 def predict(self) -> dict:
71     """
72     blocking command that runs pytorch model inference
73     """
74     intensity = self._input_data["intensity"]
75     scattering_angle = self._input_data["tth"]
76     attenuation = self._input_data["transm"]
77     priors = self._input_data["priors"]
78
79     preprocess_params = {
80         "wavelength": energy_to_wavelength(
81             self._preprocess_data["energy_keV"] * 1000
82         ),
83         "beam_width": self._preprocess_data["beam_width"],
84         "sample_length": self._preprocess_data["sample_length"],
85     }
86
87     self.inference_model.set_preprocessing_parameters(**
88 preprocess_params)
89
90     res_dict = self.inference_model.predict(
91         intensity, scattering_angle, attenuation, priors,
92     )
93
94     pprint(res_dict)
95
96     self.prediction_output["q"] = res_dict["q_values"]
97     self.prediction_output["q_interp"] = res_dict["q_interp"]
98     self.prediction_output["refl"] = res_dict["curve"]
99     self.prediction_output["refl_interp"] = res_dict["curve_interp"]

```

```

]
99     self.prediction_output["refl_predicted"] = res_dict["
curve_predicted"]
100     self.prediction_output["parameters"] = res_dict["params"]
101     self.prediction_output["sld_profile"] = res_dict["sld_profile"]
102     self.prediction_output["sld_x_axis"] = res_dict["sld_x_axis"]
103     self.prediction_output["parameter_names"] = res_dict["
param_names"]
104
105     self.prediction_output["refl_predicted_polished"] = res_dict["
curve_polished"]
106     self.prediction_output["parameters_polished"] = res_dict["
params_polished"]
107     self.prediction_output["sld_profile_polished"] = res_dict[
"sld_profile_polished"]
108
109 ]
110
111     return 0
112
113     def _initialize_dynamic_attributes(self, prefix, attributes):
114         """
115         boiler plate code to achieve generic handling of data arrays
and
116         parameters that have to be passed into the tango server and
back
117         to the client
118         """
119
120         if prefix in self._prefix_dict:
121             att_dict = self._prefix_dict[prefix]
122         else:
123             att_dict = dict()
124
125         for k, v in attributes.items():
126             att_type = None
127
128             if isinstance(v, tuple):
129                 att_type = v[0]
130                 att_dict[k] = v[1]
131             elif isinstance(v, Iterable):
132                 att_type = v
133                 att_dict[k] = []
134             else:
135                 att_type = v
136                 att_dict[k] = None
137
138             attr = attribute(
139                 name=prefix + "_" + k,
140                 dtype=att_type,
141                 access=AttrWriteType.READ_WRITE,
142                 fget=self._generic_read,
143                 fset=self._generic_write,
144                 max_dim_x=256, # self.N_MAX_X,
145                 max_dim_y=256, # self.N_MAX_Y,
146                 # fisallowed=self.generic_is_allowed,
147

```

```

148         self.add_attribute(attr)
149
150         self._prefix_dict[prefix] = att_dict
151         return self._prefix_dict[prefix]
152
153     def _generic_read(self, attr):
154         prefix, name = attr.get_name().split("_", 1)
155         value = self._prefix_dict[prefix][name]
156         # unlike a normal static attribute read, one has to modify the
157         # value
158         # inside this attr object, rather than just returning the value
159         attr.set_value(value)
160
161     def _generic_write(self, attr):
162         prefix, name = attr.get_name().split("_", 1)
163         self._prefix_dict[prefix][name] = attr.get_write_value()
164
165 if __name__ == "__main__":
166     run((TorchEvaluator,))

```

## SI-2. Beamline / BLISS integration to run ML inference on remote tango device server and publish prediction results together with raw data

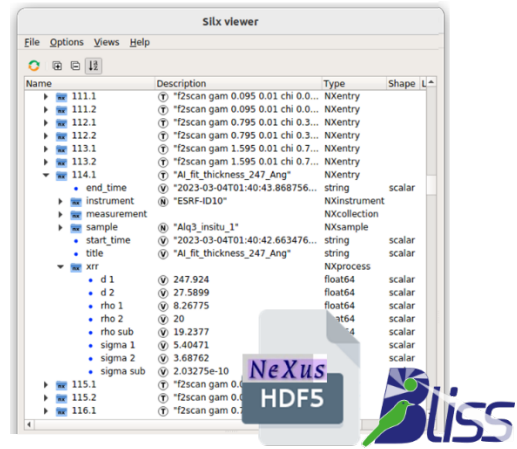

Fig. SI-1.: NeXus compliant data file generated by the beamline control system including results of the online data analysis.

Script that can be loaded as BLISS user macro into the beamline software environment without any additional external dependencies. The function `predict_and_save` takes a bliss scan object as input, runs ML inference and processes the results so that they are saved together with the raw data in a coherent fashion.

## References:

[https://bliss.gitlab-pages.esrf.fr/bliss/1.10.x/scan\\_group.html#sequences](https://bliss.gitlab-pages.esrf.fr/bliss/1.10.x/scan_group.html#sequences)

(accessed: 05.2023)

[https://bliss.gitlab-pages.esrf.fr/bliss/1.10.x/data/data\\_scan\\_metadata.](https://bliss.gitlab-pages.esrf.fr/bliss/1.10.x/data/data_scan_metadata.html)

html (accessed: 05.2023)

```

1 import numpy as np
2 from dataclasses import dataclass
3
4 from bliss.common import tango
5 from bliss import setup_globals
6 from bliss.scanning.group import Sequence
7 from bliss.scanning.chain import AcquisitionChannel
8 from bliss.scanning.scan_meta import USER_SCAN_META
9
10 # Add XRR Metadata entry to BLISS
11 if "xrr" not in USER_SCAN_META.categories_names():
12     USER_SCAN_META.add_categories({"xrr"})
13     USER_SCAN_META.xrr.set("xrr", {"@NX_class": "NXprocess"})
14
15
16 @dataclass
17 class Priors:
18     d_top: tuple = (0.0, 1000.0)
19     d_sio2: tuple = (10.0, 30.0)
20
21     sigma_top: tuple = (0.0, 50.0)
22     sigma_sio2: tuple = (
23         0.0,
24         10.0,
25     )
26     sigma_si: tuple = (
27         0.0,
28         2.0,
29     )
30
31     rho_top: tuple = (7.0, 14.0)
32     rho_sio2: tuple = (19, 23)
33     rho_si: tuple = (19, 21)
34     max_d_change: float = 5.0
35     fit_growth: bool = True
36
37     def to_arr(self):
38         return np.array(
39             [
40                 self.d_top,
41                 self.d_sio2,
42                 self.sigma_top,
43                 self.sigma_sio2,
44                 self.sigma_si,

```

```

45         self.rho_top,
46         self.rho_sio2,
47         self.rho_si,
48     ]
49 )
50
51
52 @dataclass
53 class PreprocessParams:
54     energy_keV: float = 17.0
55     beam_width: float = 0.03
56     sample_length: float = 9.0
57
58
59 def predict_and_save(
60     scans, priors=None, preprocess: PreprocessParams = None,
61 ):
62     """
63     takes a list of scans that will be concatenated to a single XRR
64     profile,
65     preforms basic background correction, pushes data via TANGO into
66     the ML model,
67     triggers inference in the TANGO device, retrieves prediction
68     results and
69     publishes results via BLISS to be saved together with original
70     scans in
71     the NeXus hdf5 file produced by the BLISS NeXusWriter
72     """
73
74     # specify the tango uri of the device server embedding the ML-Model
75     tango_uri_or_proxy = ("//VISA-HOST.esrf.fr:PORT/PATH/TO/TANGO-ML-
76     DEVICE",)
77
78     # specify counters that should be used to collect the data from the
79     scan object
80     TTH = setup_globals.gam # gam: angle of detector axis
81     CROI = "pilatus300k:roi_counters:roi2_sum" # ROI with specular
82     signal
83     BGROI1 = (
84         "pilatus300k:roi_counters:roi3_sum" # ROI left of CROI (half
85         the size of CROI)
86     )
87     BGROI2 = (
88         "pilatus300k:roi_counters:roi4_sum" # ROI right of CROI (half
89         the size of CROI)
90     )
91     TRANSM = "autof_eh1:transm" # transmission of Autoabsorber
92
93     # extract detector angle from scans
94     tth_data = np.concatenate(np.array([x.get_data(TTH) for x in scans
95     ]))
96
97     # extract transmission of attenuators from scans
98     transm_data = np.concatenate(np.array([x.get_data(TRANSM) for x in
99     scans]))

```

```

90 # extract measured intensities from scans and perform basic
    background correction
91 intens_data = np.concatenate(
92     np.array(
93         [x.get_data(CROI) - x.get_data(BGROI1) - x.get_data(BGROI2)
94          for x in scans]
95     )
96 )
97 # establish communication with tango device that is linked to ML
    model
98 ml_device = tango.DeviceProxy(tango_uri_or_proxy)
99
100 # deal with priors and preprocessing parameters
101 priors = priors or Priors()
102 preprocess = preprocess or PreprocessParams()
103
104 # push data to tango device
105 ml_device.input_tth = tth_data
106 ml_device.input_transm = transm_data
107 ml_device.input_intensity = np.clip(intens_data, 0, np.infty)
108 ml_device.input_count_time = [0]
109 ml_device.input_priors = priors.to_arr()
110 ml_device.postprocess_max_d_change = priors.max_d_change
111 ml_device.postprocess_fit_growth = priors.fit_growth
112 ml_device.preprocess_beam_width = preprocess.beam_width
113 ml_device.preprocess_sample_length = preprocess.sample_length
114 ml_device.preprocess_energy_keV = preprocess.energy_keV
115
116 # run inference (here built to run synchronous in blocking fashion)
117 ml_device.set_timeout_millis(5000)
118 ml_device.predict()
119
120 # retrieve predicted parameters
121 # polished parameters refers to results of subsequent LMS fit after
    inference
122 polished_params = ml_device.prediction_parameters_polished
123 param_names = ml_device.prediction_parameter_names
124
125 # create summary metadata structure that is to be published via
    BLISS
126 info = {"xrr": dict(zip(param_names, polished_params))}
127
128 # creates a new entry in the hdf5 file generated by BLISS and redis
    DB for online access
129 seq = Sequence(
130     title=f"AI_fit_thickness_{int(polished_params[0])}_Ang",
    scan_info=info
131 )
132
133 # specify additional data entries that should appear under "
    measurement" in the h5 file
134 seq.add_custom_channel(AcquisitionChannel("raw_tth", float, ()))
135 seq.add_custom_channel(AcquisitionChannel("corrected_intensity",
    float, ()))
136 seq.add_custom_channel(AcquisitionChannel("raw_q", float, ()))

```

```

137     seq.add_custom_channel(AcquisitionChannel("predicted_intensity",
138         float, ()))
139     seq.add_custom_channel(AcquisitionChannel("predicted_q", float, ()))
140     seq.add_custom_channel(AcquisitionChannel("params", float, ()))
141     seq.add_custom_channel(AcquisitionChannel("params_names", str, ()))
142     seq.add_custom_channel(AcquisitionChannel("polished_intensity",
143         float, ()))
144     seq.add_custom_channel(AcquisitionChannel("polished_params", float,
145         ()))
146
147     # add references to the raw data scans as well as process data and
148     # analysis results
149     with seq.sequence_context() as scan_seq:
150         for scan in scans:
151             scan_seq.add(scan)
152
153             seq.custom_channels["raw_tth"].emit(tth_data)
154             seq.custom_channels["corrected_intensity"].emit(ml_device.
155 prediction_refl)
156             seq.custom_channels["raw_q"].emit(ml_device.prediction_q)
157             seq.custom_channels["predicted_intensity"].emit(
158                 ml_device.prediction_refl_predicted
159             )
160             seq.custom_channels["params"].emit(ml_device.
161 prediction_parameters)
162             seq.custom_channels["params_names"].emit(ml_device.
163 prediction_parameter_names)
164             seq.custom_channels["polished_intensity"].emit(
165                 ml_device.prediction_refl_predicted_polished
166             )
167             seq.custom_channels["polished_params"].emit(polished_params)
168
169     # return polished_params e.g. for closed loop feedback
170     return polished_params

```

### SI-3. Asynchronous BLISS integration to receive events via the BLISS data streaming API

The code snippet below represents basically a consumer of events emitted via the event based data streaming api of BLISS and publishes produced results using a beacon channel.

References: [https://bliss.gitlab-pages.esrf.fr/bliss/1.10.x/data/data\\_redis\\_api\\_low.html](https://bliss.gitlab-pages.esrf.fr/bliss/1.10.x/data/data_redis_api_low.html) (accessed: 05.2023)

[https://bliss.gitlab-pages.esrf.fr/bliss/1.10.x/beacon\\_channels.html](https://bliss.gitlab-pages.esrf.fr/bliss/1.10.x/beacon_channels.html) (accessed: 05.2023)

```

1 from bliss.data.node import get_session_node
2 from bliss.config.channels import Channel
3
4 # create BLISS Channel with unique name in the scope of the beamline
5 # to publish predictions results via beacon / redis
6 last_film_thickness = Channel("last_film_thickness", default_value=None
7                                )
8
9 def listen_scans_of_session(session):
10     """
11     script that can run in any bliss process
12     (independent of the process producing the data & controlling the
13     hardware)
14     takes as input argument the name of the bliss session publishing
15     the data
16     to the beamline beacon server / redis
17     """
18
19     session_node = get_session_node(session)
20     print(f"Listening to {session}")
21
22     received_scans = []
23     for event_type, node, event_data in session_node.walk_on_new_events(
24         include_filter=["scan"]
25     ):
26         # this loop deals with the event based data streaming api of
27         # BLISS
28         #
29         if event_type == event_type.NEW_NODE:
30             print(f"new scan", node.db_name)
31
32         elif event_type == event_type.END_SCAN:
33             print(node.db_name)
34
35             params = node.info.get("fastfit")
36             if params.get("xrr_scan_group_first", False):
37                 received_scans = [node]
38                 print("add scan")
39             if params.get("xrr_scan_group_last", False):
40                 received_scans.append(node)
41                 print("add scan and process")
42                 process_scans(received_scans)
43
44 def process_scans(scans):
45     """
46     Run ML inference
47     """
48
49     # missing here: code similar to synchronous version in example
50     # above
51     # interacting with tango or triton server to retrieve prediction
52     # ...

```

```

51     thickness = prediction["parameters_polished"][0]
52
53
54     # publish e.g. film thickness via bliss channel & beacon
55     # to make it available to all bliss processes running on the
    beamline
56     last_film_thickness.value = thickness
57
58     print("##### predicted thickness", thickness)

```

#### SI-4. Postprocessing gradient-descent fit with optional growth rate parameter.

The functions below are used to perform a postprocessing polishing operation by fitting the measured curve via gradient descent initialized based on AI result. Optionally, it allows fitting the linear change of the thickness of the top layer as a function of  $q$  for curves measured *in situ* during growth. Further details may be found in (Munteanu *et al.*, 2023).

References:

Munteanu, V., Starostin, V., Greco, A., Pithan, L., Gerlach, A., Hinderhofer, A., Kowarik, S. Schreiber, F. (2023). Neural network analysis of neutron and X-ray reflectivity data: incorporating prior knowledge for tackling the phase problem.

```

1 import numpy as np
2 from scipy.optimize import minimize, curve_fit
3
4 def abeles_np(
5     q: np.ndarray,
6     thickness: np.ndarray,
7     roughness: np.ndarray,
8     sld: np.ndarray):
9
10     c_dtype = np.complex128 if q.dtype is np.float64 else np.complex64
11
12     if q.ndim == thickness.ndim == roughness.ndim == sld.ndim == 1:
13         zero_batch = True
14     else:
15         zero_batch = False
16

```

```

17 thickness = np.atleast_2d(thickness)
18 roughness = np.atleast_2d(roughness)
19 sld = np.atleast_2d(sld)
20 batch_size, num_layers = thickness.shape
21 sld = np.concatenate([np.zeros((batch_size, 1)).astype(sld.dtype),
22 sld], -1)[: , None]
23 thickness = np.concatenate([np.zeros((batch_size, 1)).astype(
24 thickness.dtype), thickness], -1)[: , None]
25 roughness = roughness[: , None] ** 2
26
27 sld = sld * 1e-6 + 1e-30j
28
29 k_z0 = (q / 2).astype(c_dtype)
30 if len(k_z0.shape) == 1:
31     k_z0 = k_z0[None]
32 if len(k_z0.shape) == 2:
33     k_z0 = k_z0[... , None]
34 k_n = np.sqrt(k_z0 ** 2 - 4 * np.pi * sld)
35 k_n, k_np1 = k_n[... , :-1], k_n[... , 1:]
36
37 beta = 1j * thickness * k_n
38
39 exp_beta = np.exp(beta)
40 exp_m_beta = np.exp(-beta)
41 rn = (k_n - k_np1) / (k_n + k_np1) * np.exp(- 2 * k_n * k_np1 *
42 roughness)
43
44 c_matrices = np.stack([
45     np.stack([exp_beta, rn * exp_m_beta], -1),
46     np.stack([rn * exp_beta, exp_m_beta], -1),
47 ], -1)
48 c_matrices = np.moveaxis(c_matrices, -3, 0)
49 m, c_matrices = c_matrices[0], c_matrices[1:]
50 for c in c_matrices:
51     m = m @ c
52
53 r = np.abs(m[... , 1, 0] / m[... , 0, 0]) ** 2
54 r = np.clip(r, None, 1.)
55
56 if zero_batch:
57     r = r[0]
58 return r
59
60 def standard_restore_params(fitted_params) -> dict:
61     num_layers = (fitted_params.size - 2) // 3
62     return dict(
63         thickness=fitted_params[:num_layers],
64         roughness=fitted_params[num_layers:2 * num_layers + 1],
65         sld=fitted_params[2 * num_layers + 1:],
66     )
67
68 def mse_loss(curve1, curve2):
69     return np.sum((curve1 - curve2) ** 2)

```

```

70
71 def standard_refl_fit(
72     q: np.ndarray, curve: np.ndarray,
73     init_params: np.ndarray,
74     bounds: np.ndarray = None,
75     refl_generator=abeles_np,
76     restore_params_func=standard_restore_params,
77     scale_curve_func=np.log10,
78     **kwargs):
79
80     if bounds is not None:
81         kwargs['bounds'] = bounds
82         init_params = np.clip(init_params, *bounds)
83
84     res = curve_fit(
85         get_scaled_curve_func(
86             refl_generator=refl_generator,
87             restore_params_func=restore_params_func,
88             scale_curve_func=scale_curve_func,
89         ),
90         q, scale_curve_func(curve),
91         p0=init_params, **kwargs
92     )
93
94     curve = refl_generator(q, **restore_params_func(res[0]))
95     return res[0], curve
96
97
98 def get_fit_with_growth(
99     q: np.ndarray, curve: np.ndarray,
100     init_params: np.ndarray,
101     bounds: np.ndarray = None,
102     init_d_change: float = 0.,
103     max_d_change: float = 30.,
104     scale_curve_func=np.log10,
105     **kwargs):
106
107     init_params = np.array(list(init_params) + [init_d_change])
108     if bounds is not None:
109         bounds = np.concatenate([bounds, np.array([0, max_d_change])
110     [..., None]], -1)
111
112     params, curve = standard_refl_fit(
113         q, curve, init_params, bounds, refl_generator=
114         refl_with_changing_params,
115         restore_params_func=get_restore_params_with_growth_func(q_size=
116         q.size, d_idx=0),
117         scale_curve_func=scale_curve_func, **kwargs
118     )
119     params[0] += params[-1] / 2
120     return params, curve
121
122 def fit_refl_curve(q: np.ndarray, curve: np.ndarray,
123     init_params: np.ndarray,
124     bounds: np.ndarray = None,

```

```

123         refl_generator=abeles_np,
124         restore_params_func=standard_restore_params,
125         scale_curve_func=np.log10,
126         **kwargs
127     ) -> np.ndarray
128
129     fitting_func = get_fitting_func(
130         q=q, curve=curve,
131         refl_generator=refl_generator,
132         restore_params_func=restore_params_func,
133         scale_curve_func=scale_curve_func,
134     )
135
136     res = minimize(fitting_func, init_params, bounds=bounds, **kwargs)
137
138     if not res.success:
139         import warnings
140         warnings.warn(f"Minimization did not converge.")
141     return res.x
142
143
144 def get_scaled_curve_func(
145     refl_generator=abeles_np,
146     restore_params_func=standard_restore_params,
147     scale_curve_func=np.log10):
148
149     def scaled_curve_func(q, *fitted_params):
150         fitted_params = restore_params_func(np.asarray(fitted_params))
151         fitted_curve = refl_generator(q, **fitted_params)
152         scaled_curve = scale_curve_func(fitted_curve)
153         return scaled_curve
154
155     return scaled_curve_func
156
157
158 def get_fitting_func(
159     q: np.ndarray,
160     curve: np.ndarray,
161     refl_generator=abeles_np,
162     restore_params_func=standard_restore_params,
163     scale_curve_func=np.log10,
164     loss_func=mse_loss):
165
166     scaled_curve = scale_curve_func(curve)
167
168     def fitting_func(fitted_params):
169         fitted_params = restore_params_func(fitted_params)
170         fitted_curve = refl_generator(q, **fitted_params)
171         loss = loss_func(scale_curve_func(fitted_curve), scaled_curve)
172         return loss
173
174     return fitting_func
175
176
177 def restore_masked_params(fixed_params, fixed_mask):
178     def restore_params(fitted_params) -> dict:

```

```

179     params = np.empty_like(fixed_mask).astype(fitted_params.dtype)
180     params[fixed_mask] = fixed_params
181     params[~fixed_mask] = fitted_params
182     return standard_restore_params(params)
183
184     return restore_params
185
186
187 def base_params2growth(base_params: dict, d_shift: np.ndarray, d_idx:
188     int = 0) -> dict:
189     d_init = base_params['thickness'][None]
190     q_size = d_shift.size
191     d = d_init.repeat(q_size, 0)
192     d[:, d_idx] = d[:, d_idx] + d_shift
193
194     roughness = np.broadcast_to(base_params['roughness'][None], (q_size
195     , base_params['roughness'].size))
196     sld = np.broadcast_to(base_params['sld'][None], (q_size,
197     base_params['sld'].size))
198
199     return {
200         'thickness': d,
201         'roughness': roughness,
202         'sld': sld,
203     }
204
205 def get_restore_params_with_growth_func(q_size: int, d_idx: int = 0):
206     def restore_params_with_growth(fitted_params) -> dict:
207         fitted_params, delta_d = fitted_params[:-1], fitted_params[-1]
208         base_params = standard_restore_params(fitted_params)
209         d_shift = np.linspace(0, delta_d, q_size)
210         return base_params2growth(base_params, d_shift, d_idx)
211
212     return restore_params_with_growth
213
214 def refl_with_changing_params(q: np.ndarray, **kwargs):
215     return abeles_np(q[..., None], **kwargs).flatten()

```
